# Supplementary material for: Enhanced Twist-Averaging Technique for Magnetic Metals: Applications using Quantum Monte Carlo
Source: arXiv:2401.06926 ancillary file (2024-03-19)
Supplement: Supplementary file 1 [file gcta_supplemental.pdf]

# Supplementary Information for “Enhanced Twist-Averaging Technique for Magnetic Metals: Applications using Quantum Monte Carlo”

Abdulgani Annaberdiyev,<sup>1</sup> Panchapakesan Ganesh,<sup>1</sup> and Jaron T. Krogel<sup>2</sup>

<sup>1</sup>*Center for Nanophase Materials Sciences, Oak Ridge National Laboratory, Oak Ridge, Tennessee 37831, USA\**

<sup>2</sup>*Materials Science and Technology Division, Oak Ridge National Laboratory, Oak Ridge, Tennessee 37831, USA†*

## SUPPLEMENTARY SECTION 1. BULK GEOMETRIES

### A. Al

This Supplementary Subsection provides the bulk geometry for the face-centered-cubic (FCC) Al as shown in Figure 1a. We use the experimental lattice parameter [1] extrapolated to  $T = 0$  K. The structure is provided in Table 1 in the **xsf** format.

Supplementary Table 1: Employed bulk geometry of FCC Al in **xsf** format (Å units). The lattice parameter is  $a = 4.0317(2)$  Å. The space group is  $Fm\bar{3}m$  (#225).

|           |              |              |              |
|-----------|--------------|--------------|--------------|
| CRYSTAL   |              |              |              |
| PRIMVEC   |              |              |              |
|           | 4.0317000000 | 0.0000000000 | 0.0000000000 |
|           | 0.0000000000 | 4.0317000000 | 0.0000000000 |
|           | 0.0000000000 | 0.0000000000 | 4.0317000000 |
| PRIMCOORD |              |              |              |
| 4         | 1            |              |              |
| 13        | 0.0000000000 | 0.0000000000 | 0.0000000000 |
| 13        | 2.0158500000 | 2.0158500000 | 0.0000000000 |
| 13        | 0.0000000000 | 2.0158500000 | 2.0158500000 |
| 13        | 2.0158500000 | 0.0000000000 | 2.0158500000 |

### B. $\alpha$ -Fe

This Supplementary Subsection provides the bulk geometry for  $\alpha$ -Fe, which has a body-centered-cubic (BCC) structure as shown in Figure 1b. We use the experimental lattice parameter [2] extrapolated to  $T = 0$  K. The structure is provided in Table 2 in the **xsf** format.

Supplementary Table 2: Employed bulk geometry of BCC  $\alpha$ -Fe in **xsf** format (Å units). The lattice parameter is  $a = 2.8598$  Å. The space group is  $Im\bar{3}m$  (#229).

|           |              |              |              |
|-----------|--------------|--------------|--------------|
| CRYSTAL   |              |              |              |
| PRIMVEC   |              |              |              |
|           | 2.8598000000 | 0.0000000000 | 0.0000000000 |
|           | 0.0000000000 | 2.8598000000 | 0.0000000000 |
|           | 0.0000000000 | 0.0000000000 | 2.8598000000 |
| PRIMCOORD |              |              |              |
| 2         | 1            |              |              |
| 26        | 0.0000000000 | 0.0000000000 | 0.0000000000 |
| 26        | 1.4299000000 | 1.4299000000 | 1.4299000000 |

\* annaberdiyea@ornl.gov

† krogeljt@ornl.gov

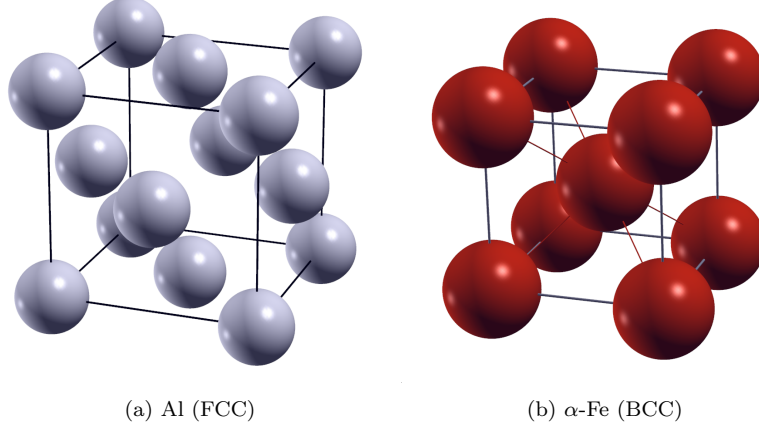

Supplementary Figure 1: (a) The face-centered-cubic (FCC) structure of Al (4 Al atoms), (b) the body-centered-cubic (BCC) structure of  $\alpha$ -Fe (2 Fe atoms). These images were created using **XCrySDen** [3].

## SUPPLEMENTARY SECTION 2. DFT METHODS AND DATA

### A. $k$ -Mesh Convergence

This Supplementary Subsection demonstrates the  $k$ -mesh convergence in DFT for the considered materials. Tabulated quantities are the total energy, the Fermi level, Löwdin atomic moments, total cell magnetization  $M_{\text{tot}}$ , and absolute cell magnetization  $M_{\text{abs}}$ , which are defined as:

$$M_{\text{tot}} = \int_{\text{cell}} (n_{\uparrow} - n_{\downarrow}) d^3r \quad (1)$$

$$M_{\text{abs}} = \int_{\text{cell}} |n_{\uparrow} - n_{\downarrow}| d^3r. \quad (2)$$

Supplementary Table 3: Convergence of various quantities with respect to  $k$ -mesh for FCC Al (4 atoms) and BCC Fe (2 atoms).  $E_c = 400$  Ry kinetic energy cutoff and  $\sigma_e = 10^{-3}$  Ry Fermi-Dirac spreading were used. LDA functional was used for Al while LDA+ $U$  (5.5 eV) was used for  $\alpha$ -Fe.  $E_F$  is the Fermi level,  $\mu$  is the Löwdin atomic moment,  $M_{\text{tot}} = \int_{\text{cell}} (n_{\uparrow} - n_{\downarrow}) d^3r$  is the total cell magnetization, and  $M_{\text{abs}} = \int_{\text{cell}} |n_{\uparrow} - n_{\downarrow}| d^3r$  is the absolute cell magnetization. All values were determined self-consistently.  $[24 \times 24 \times 24]$   $k$ -mesh was used for SCF throughout the work.

| $k$ -mesh                  | Total Energy [Ry] | $E_F$ [eV] | $\mu_1$ [ $\mu_B$ ] | $\mu_2$ [ $\mu_B$ ] | $M_{\text{tot}}$ [ $\mu_B$ ] | $M_{\text{abs}}$ [ $\mu_B$ ] |
|----------------------------|-------------------|------------|---------------------|---------------------|------------------------------|------------------------------|
| Al (NM)                    |                   |            |                     |                     |                              |                              |
| $[6 \times 6 \times 6]$    | -16.51634307      | 7.9290     |                     |                     |                              |                              |
| $[12 \times 12 \times 12]$ | -16.50979062      | 8.1316     |                     |                     |                              |                              |
| $[18 \times 18 \times 18]$ | -16.51041406      | 8.1688     |                     |                     |                              |                              |
| $[24 \times 24 \times 24]$ | -16.51051170      | 8.1650     |                     |                     |                              |                              |
| $\alpha$ -Fe (FM)          |                   |            |                     |                     |                              |                              |
| $[6 \times 6 \times 6]$    | -493.83175370     | 17.4248    | 3.0709              | 3.0708              | 5.8114                       | 6.1011                       |
| $[12 \times 12 \times 12]$ | -493.83174720     | 17.4211    | 3.0471              | 3.0470              | 5.6680                       | 6.0648                       |
| $[18 \times 18 \times 18]$ | -493.83139192     | 17.3962    | 3.0343              | 3.0343              | 5.6335                       | 6.0373                       |
| $[24 \times 24 \times 24]$ | -493.83150610     | 17.4098    | 3.0434              | 3.0434              | 5.6583                       | 6.0577                       |

Table 3 provides the convergence with respect to  $k$ -mesh for various DFT quantities of the considered materials. Note that all quantities are converged at  $[24 \times 24 \times 24]$   $k$ -mesh, which is the mesh used throughout the work. Also, note that the atomic moments can be reliably obtained using the  $M_{\text{abs}}$ :

$$\mu = \frac{M_{\text{abs}}}{2} \quad (3)$$

which provides values in close agreement with the Löwdin atomic moments.

## B. Band Structures

This Supplementary Subsection provides the band structures for the considered materials. The high symmetry points in the Brillouin zone path are shown in Figure 2. The band structures are shown in Figure 3. The results are obtained using a converged  $k$ -mesh of  $[24 \times 24 \times 24]$ . LDA was used for Al, while LDA+ $U$ (5.5 eV) was used for  $\alpha$ -Fe.

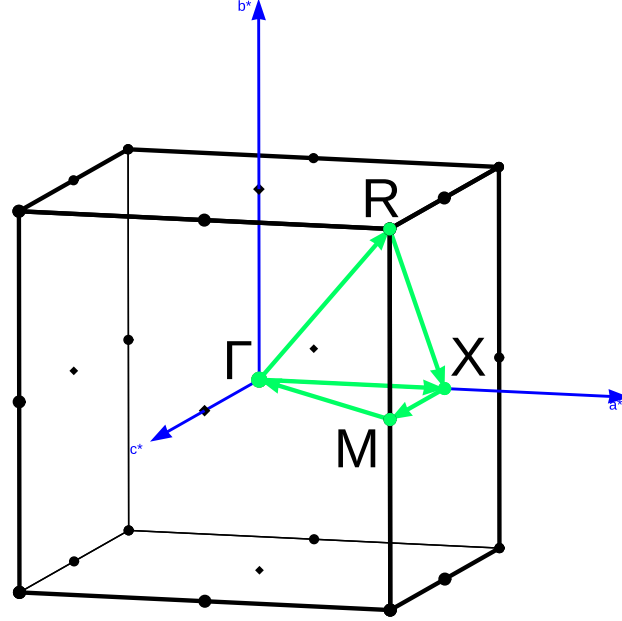

Supplementary Figure 2: High symmetry points in the Brillouin zone of the cubic lattice employed in Al and  $\alpha$ -Fe. This image was created using **XCrySDen** [3].

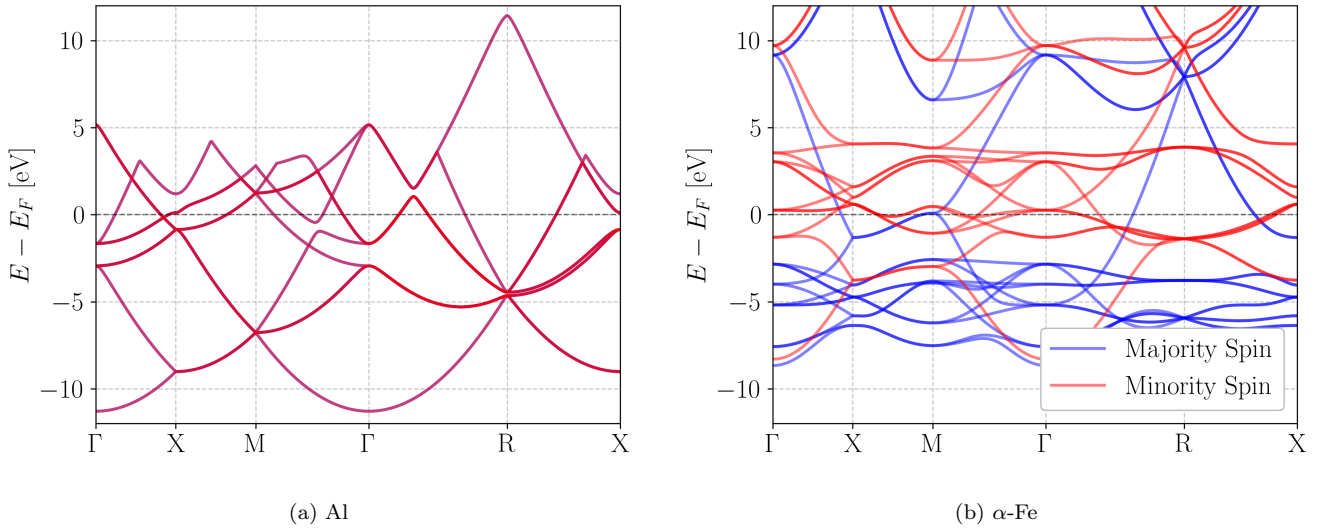

Supplementary Figure 3: Band structures for the considered materials. (a) Al in NM phase using LDA, (b)  $\alpha$ -Fe in FM phase using LDA+ $U$ (5.5 eV).

### C. Density of States

This Supplementary Subsection provides the density of states (DOS) for the considered materials, as shown in Figure 4. The results are obtained using a converged  $k$ -mesh of  $[24 \times 24 \times 24]$ . LDA was used for Al, while LDA+ $U$ (5.5 eV) was used for  $\alpha$ -Fe.

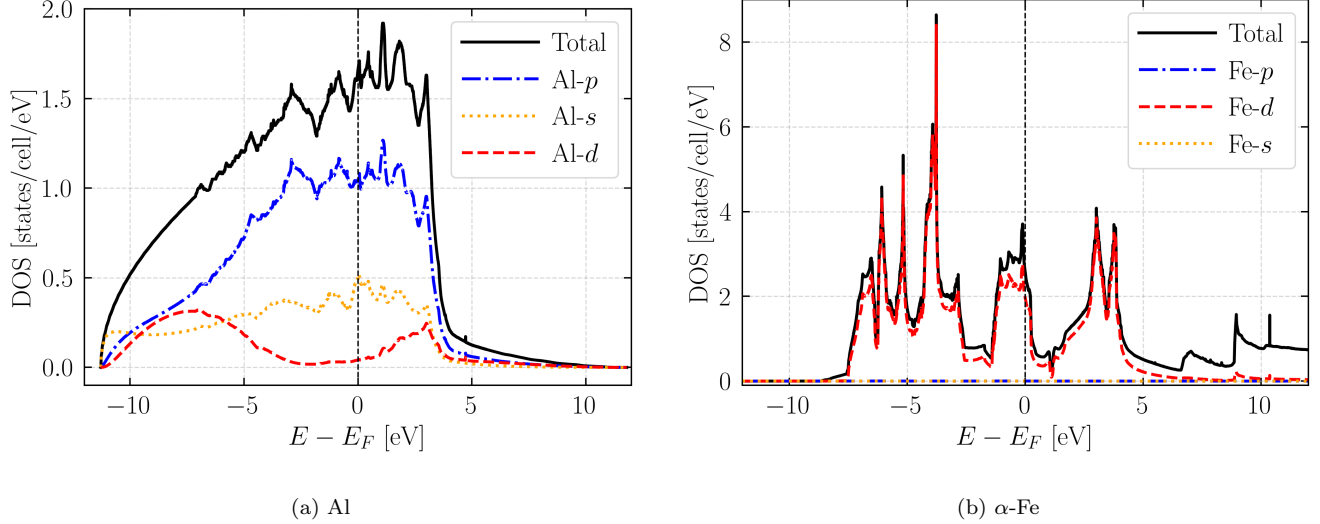

Supplementary Figure 4: Density of states for the considered materials. (a) Al in NM phase using LDA, (b)  $\alpha$ -Fe in FM phase using LDA+ $U$ (5.5 eV).

### D. Pseudopotential Bias

This Supplementary Subsection provides data on the role of pseudopotential accuracy. Table 4 shows the Al cohesive energies using ccECP and Troullier-Martins (TM) pseudopotential. The TM pseudopotential was generated using **Opium** with PBE functional and is not the same potential used by Ref. [4]. Therefore, the difference between ccECP and TM represents only a qualitative difference, such as an underestimation or overestimation tendency. From this data, we see a qualitative tendency of TM pseudopotential to underestimate the cohesive energy of fcc Al.

Supplementary Table 4: Comparison of Al cohesive energies [eV] using ccECP versus Troullier-Martins (TM) pseudopotentials.  $\Delta E_{\text{coh}}$  is the difference between ccECP and TM values.

| DFT Functional | ccECP [eV] | TM [eV]  | $\Delta E_{\text{coh}}$ [eV] |
|----------------|------------|----------|------------------------------|
| LDA            | 3.884      | 3.615    | 0.269                        |
| PBE            | 3.451      | 3.187    | 0.264                        |
| DMC/SJ         | 3.437(3)   | 3.071(4) | 0.366(5)                     |

## SUPPLEMENTARY SECTION 3. QMC METHODS AND DATA

### A. DMC Time Step Convergence

This Supplementary Subsection provides the convergence plots for the DMC time step in the considered materials. Figure 5 shows the total and kinetic energies as the DMC time step is varied.  $[2 \times 2 \times 2]$  supercells at  $k = \Gamma$  were employed for both Al and Fe. We used  $\tau = 5 \times 10^{-3} \text{ Ha}^{-1}$  time step throughout the work, which results in acceptance ratios larger than 99% in both cases. The acceptance ratios and the energy differences between the time step extrapolated energy and the chosen time step energy are provided in Table 5.

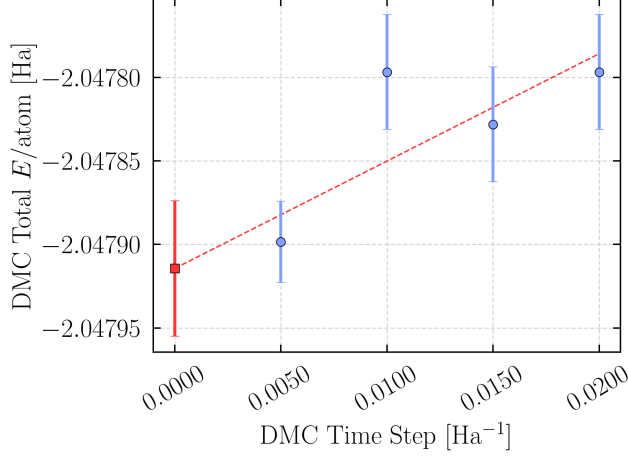

(a) Al Total Energy

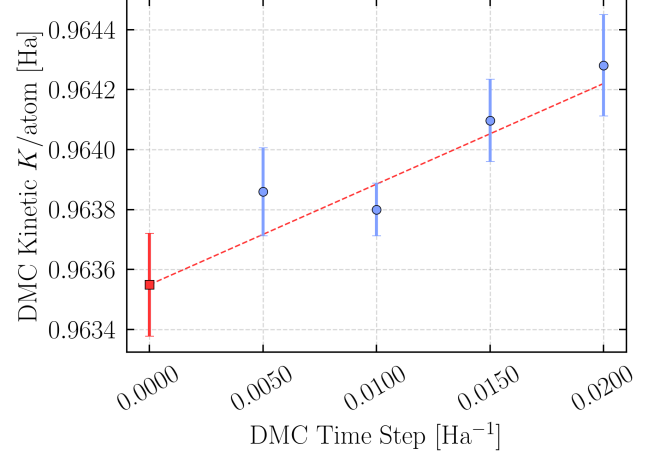

(b) Al Kinetic Energy

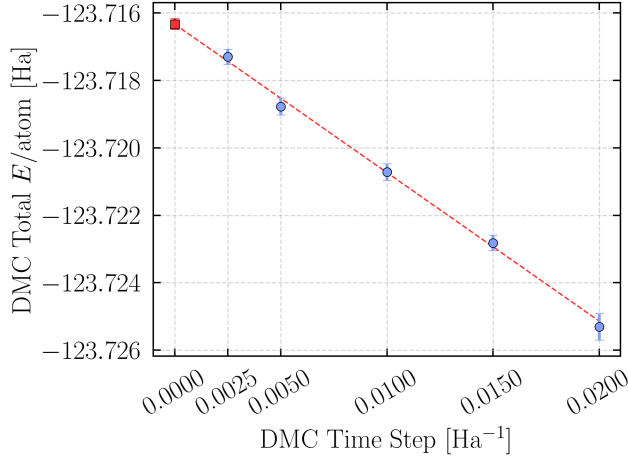

(c) Fe Total Energy

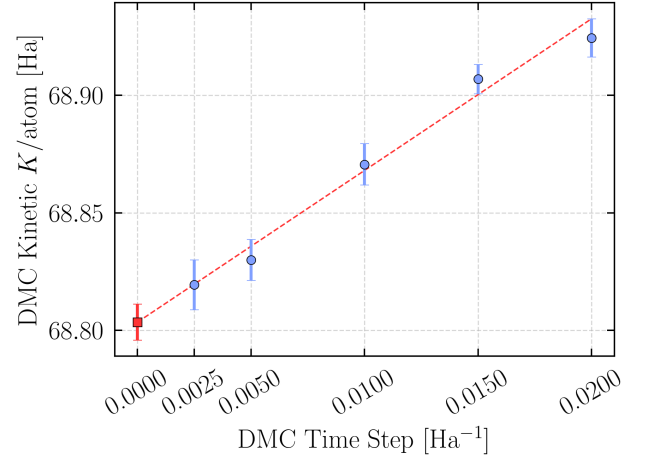

(d) Fe Kinetic Energy

Supplementary Figure 5: DMC time step convergence for Al and  $\alpha$ -Fe. Total and kinetic energies are shown for (a, b) Al (32 atoms) and (c, d)  $\alpha$ -Fe (16 atoms).

Supplementary Table 5: DMC time step convergence for Al and  $\alpha$ -Fe. Acceptance ratios [%] are shown for each case.  $\Delta E = (E_0 - E_\tau)$  and  $\Delta K = (K_0 - K_\tau)$  are total and kinetic energy differences between the time step extrapolated energy and the chosen time step energy, respectively.

| Material     | Acceptance [%] | $\Delta E$ [Ha] | $\Delta K$ [Ha] |
|--------------|----------------|-----------------|-----------------|
| Al           | 99.97          | -0.00002(5)     | -0.0003(2)      |
| $\alpha$ -Fe | 99.18          | 0.0025(3)       | -0.03(1)        |

## B. QMC Charge and Moment Evaluation

Let  $\rho_\uparrow(r)/\rho_\downarrow(r)$  be the up/down channel densities obtained in QMC. These densities are accumulated as a histogram in a defined  $[100 \times 100 \times 100]/(\text{primitive cell})$  3D grid:

$$\rho_{\uparrow/\downarrow}^{\text{QMC}}(\mathbf{r}) = \sum_i^{M_{\uparrow/\downarrow}} \frac{\delta(\mathbf{r} - \mathbf{r}_i)}{\Omega^3} \quad (4)$$

where  $\Omega^3$  is the grid volume and  $M_{\uparrow/\downarrow}$  is the number of up/down electrons within  $\Omega^3$ . Then, the cumulative charge densities, namely, the atomic occupations, are calculated as follows:

$$q = \int_{r=0}^{R_c} [\rho_{\uparrow}(r) + \rho_{\downarrow}(r)] 4\pi r^2 dr. \quad (5)$$

The cumulative spin densities, namely, the magnetic moments, are calculated as follows:

$$\mu = \int_{r=0}^{R_c} [\rho_{\uparrow}(r) - \rho_{\downarrow}(r)] 4\pi r^2 dr. \quad (6)$$

Throughout this work, we chose the cutoff radius  $R_c$  as the middle point between the two nearest-neighbor atoms:

$$R_c^{\text{Al}} = \frac{a_{\text{lattice}} \cdot \sqrt{2}}{4} = 1.425421 \text{ \AA}, \quad (7)$$

$$R_c^{\text{Fe}} = \frac{a_{\text{lattice}} \cdot \sqrt{3}}{4} = 1.238330 \text{ \AA}. \quad (8)$$

Since the density does not commute with the Hamiltonian, we use the extrapolated estimators for DMC  $q$  and  $\mu$  observables [5]:

$$\langle \Phi | \hat{\rho} | \Phi \rangle \approx 2 \langle \Phi | \hat{\rho} | \Psi_T \rangle - \langle \Psi_T | \hat{\rho} | \Psi_T \rangle + \mathcal{O}[(\Phi - \Psi_T)^2] \quad (9)$$

where  $\Psi_T$  is the trial wave function and  $\Phi$  is the DMC wave function.

### C. Al Atomic Energies

Table 6 provides the isolated atomic DMC energies of Al using various nodal surfaces. We use the DMC/ROHF values in the main text.

Supplementary Table 6: Isolated atomic total and kinetic energies [Ha] using DMC. The DMC time step is  $\tau = 5 \times 10^{-3} \text{ Ha}^{-1}$ . SCF calculations for DMC were carried out using PySCF [6, 7] with cc-pV5Z basis sets.

| Method    | Total [Ha]   | Kinetic [Ha] |
|-----------|--------------|--------------|
| DMC/ROHF  | -1.93657(3)  | 0.7030(3)    |
| DMC/UHF   | -1.93629(3)  | 0.7054(3)    |
| DMC/R-PBE | -1.93656(3)  | 0.7032(3)    |
| DMC/U-PBE | -1.93649(3)  | 0.7041(3)    |
| FCI/CBS   | -1.937523(8) | 0.7063(1)    |

### D. Bulk Total Energies

This subsection provides the bulk total energies for Al and Fe. In each case, a least squares regression line fit was used for extrapolation, which was analyzed by the  $R^2$  “goodness-of-fit” metric:

$$R^2 = 1 - \frac{\sum_i (y_i - f_i)^2}{\sum_i (y_i - \bar{y}_i)^2} \quad (10)$$

where  $y_i$  are calculated data points,  $f_i$  are fitted values, and  $\bar{y}_i$  is the mean of data points. The  $R^2$  values are given in the main text, while the energies are provided here. Tables 7 and 8 provide the DMC supercell energies for various supercell sizes using the GCTA-SAFLL occupations.

Supplementary Table 7: Twist-averaged DMC total, kinetic, and potential energies [Ha] of Al for various supercell tilings  $[T \times T \times T]$  using the GCTA-SAFL occupations. In all cases,  $Z_T \cdot Z_\theta = 6^3$  is constant. LDA exchange-correlation functional was used as the trial wave function.

| Quantity  | $[1 \times 1 \times 1]$ | $[2 \times 2 \times 2]$ | $[3 \times 3 \times 3]$ | TDL         |
|-----------|-------------------------|-------------------------|-------------------------|-------------|
| Total     | -2.12108(6)             | -2.07021(2)             | -2.06503(2)             | -2.06291(3) |
| Kinetic   | 0.9242(3)               | 0.94279(7)              | 0.94616(7)              | 0.9464(8)   |
| Potential | -3.0453(3)              | -3.01300(7)             | -3.01120(8)             | -3.0092(8)  |

Supplementary Table 8: Twist-averaged DMC total, kinetic, and potential energies [Ha] of  $\alpha$ -Fe for various supercell tilings  $[T \times T \times T]$  using the GCTA-SAFL occupations. In all cases,  $Z_T \cdot Z_\theta = 6^3$  is constant. LDA+ $U$ (5.5 eV) exchange-correlation functional was used as the trial wave function.

| Quantity  | $[1 \times 1 \times 1]$ | $[2 \times 2 \times 2]$ | $[3 \times 3 \times 3]$ | TDL         |
|-----------|-------------------------|-------------------------|-------------------------|-------------|
| Total     | -123.9313(2)            | -123.7559(2)            | -123.7349(2)            | -123.729(2) |
| Kinetic   | 68.217(3)               | 68.605(4)               | 68.709(5)               | 68.69(3)    |
| Potential | -192.149(3)             | -192.361(4)             | -192.444(5)             | -192.42(3)  |

- 
- [1] P. N. H. Nakashima, *The Crystallography of Aluminum and Its Alloys* (Routledge Handbooks Online, 2018).  
[2] E. A. Owen and G. I. Williams, *Journal of Scientific Instruments* **31**, 49 (1954).  
[3] A. Kokalj, *Journal of Molecular Graphics and Modelling* **17**, 176 (1999).  
[4] R. Q. Hood, P. R. C. Kent, and F. A. Reboredo, *Physical Review B* **85**, 134109 (2012).  
[5] W. M. C. Foulkes, L. Mitas, R. J. Needs, and G. Rajagopal, *Reviews of Modern Physics* **73**, 33 (2001).  
[6] Q. Sun, T. C. Berkelbach, N. S. Blunt, G. H. Booth, S. Guo, Z. Li, J. Liu, J. D. McClain, E. R. Sayfutyarova, S. Sharma, S. Wouters, and G. K.-L. Chan, *WIREs Computational Molecular Science* **8**, e1340 (2018).  
[7] Q. Sun, X. Zhang, S. Banerjee, P. Bao, M. Barbry, N. S. Blunt, N. A. Bogdanov, G. H. Booth, J. Chen, Z.-H. Cui, J. J. Eriksen, Y. Gao, S. Guo, J. Hermann, M. R. Hermes, K. Koh, P. Koval, S. Lehtola, Z. Li, J. Liu, N. Mardirossian, J. D. McClain, M. Motta, B. Mussard, H. Q. Pham, A. Pulkin, W. Purwanto, P. J. Robinson, E. Ronca, E. R. Sayfutyarova, M. Scheurer, H. F. Schurkus, J. E. T. Smith, C. Sun, S.-N. Sun, S. Upadhyay, L. K. Wagner, X. Wang, A. White, J. D. Whitfield, M. J. Williamson, S. Wouters, J. Yang, J. M. Yu, T. Zhu, T. C. Berkelbach, S. Sharma, A. Y. Sokolov, and G. K.-L. Chan, *The Journal of Chemical Physics* **153**, 024109 (2020).
